# Supplementary material for: Understanding and Analyzing Model Robustness and Knowledge-Transfer in Multilingual Neural Machine Translation using TX-Ray
Source: arXiv:2412.13881 source file (2024-12-18)
Supplement: Supplementary file 1 [file AppendixTemplate.tex]

% Appendix Template

\chapter{Appendix Title Here} % Main appendix title

\label{AppendixX} % Change X to a consecutive letter; for referencing this appendix elsewhere, use \ref{AppendixX}

Write your Appendix content here.
